# Supplementary material for: Observing Dialogue in Therapy: Categorizing and Forecasting Behavioral Codes
Source: arXiv:1907.00326 source file (2019-06-30)
Supplement: Supplementary file 1 [file supplementary.tex]

%
% File main.tex
%
%% Based on the style files for ACL 2018, NAACL 2018/19, which were
%% Based on the style files for ACL-2015, with some improvements
%%  taken from the NAACL-2016 style
%% Based on the style files for ACL-2014, which were, in turn,
%% based on ACL-2013, ACL-2012, ACL-2011, ACL-2010, ACL-IJCNLP-2009,
%% EACL-2009, IJCNLP-2008...
%% Based on the style files for EACL 2006 by 
%%e.agirre@ehu.es or Sergi.Balari@uab.es
%% and that of ACL 08 by Joakim Nivre and Noah Smith

\documentclass[11pt,a4paper]{article}
\usepackage[hyperref]{acl2019}
\usepackage{times}
\usepackage{latexsym}

\usepackage{url}
\aclfinalcopy % Uncomment this line for the final submission
 %  Enter the acl Paper ID here

%\setlength\titlebox{5cm}
% You can expand the titlebox if you need extra space
% to show all the authors. Please do not make the titlebox
% smaller than 5cm (the original size); we will check this
% in the camera-ready version and ask you to change it back.

\usepackage{graphicx}
\usepackage{amsmath}
\usepackage{cases}
\usepackage{booktabs}
\usepackage{algorithm}
\usepackage{algorithmic}
\urlstyle{same}

\usepackage{subfig}

\usepackage{mystyle}
\usepackage{mlsymbols}

\input{common}

\graphicspath{ {images/} }
\title{\mytitle \\(Supplementary Materials)}

\author{
  Jie Cao${^\dagger}$,
  Michael Tanana${^\ddagger}$,
  Zac E. Imel${^\ddagger}$,
  Eric Poitras${^\ddagger}$,\\
  {\bf David C. Atkins}${^\diamondsuit}$,
  {\bf Vivek Srikumar}${^\dagger}$\\
  ${^\dagger}$School of Computing, University of Utah\\
  ${^\ddagger}$Department of Educational Psychology, University of Utah\\
  ${^\diamondsuit}$Department of Psychiatry and Public Health, University of Washington\\
  \texttt{\{jcao, svivek\}@cs.utah.edu,}\\
  \texttt{\{michael.tanana, zac.imel, eric.poitras\}@utah.edu,}\\
  \texttt{datkins@u.washington.edu}
 }

\date{}

\begin{document}
\maketitle

\input{appendix}

\bibliography{psyc}
\bibliographystyle{acl_natbib}

\end{document}
